# Supplementary material for: Scene Graph Reasoning with Prior Visual Relationship for Visual Question Answering
Source: arXiv:1812.09681 source file (2019-08-21)
Supplement: Supplementary file 1 [file 7_appendix.tex]

\section{Appendix}

PyTorch implementation of the models is available at \href{https://github.com/neurips19-5160/visual-relationship-encoder.pytorch}{\textit{visual-relationship-encoder.pytorch}} and \href{https://github.com/neurips19-5160/scene-gcn-vqa.pytorch}{\textit{scene-gcn-vqa.pytorch}}.

\subsection{Differences with current approaches}

The predominant approaches for VQA are based on \textit{joint embedding learning} that typically leverage CNN and LSTM to learn embeddings of images and questions respectively \cite{zhou2015simple,noh2016image, Nguyen2018improved}. These embeddings are fused by concatenation, element-wise summation/multiplication, bilinear pooling \cite{Tenebaum1997Separating,Fukui2016Multimodal,Kim2017Hadamard}, or more sophisticated fusion methods \cite{Nguyen2018improved} and then fed into a classifier for answer prediction. The problem of these approaches is that the visual features and textural features are extracted independently, which makes the visual representations difficult to adapt to the question. Several advanced works adopt the attention mechanism \cite{yang2016stacked,Nam2017CVPR,anderson2018bottom, hudson2018MAC} to focus on semantically relevant visual objects (i.e. pre-detected salient regions) according to a given question. However, these approaches treat the visual objects as isolated parts and ignore inferring the inter-object relationships.

The potential limitation of the aforementioned approaches lies in the monolithic vector representations, which fails to model and reason about the complex relational information in the visual content. Recently, implicit and explicit visual relational reasoning approaches have achieved better performance in the VQA task \cite{santoro2017simple, teney2017Graph,yi2018neural,Mascharka2018Trans,suarez2018DDRprog}. Santord \etal \cite{santoro2017simple} propose to infer the ``hidden'' relationships between all the implicit object pairs via a plug-and-play MLP module. However, it merely verifies the model's effectiveness on the limited number of  synthesized geometrical objects, which can't leverage the rich prior relational knowledge for the real-world objects. Recently, more works exploit explicit visual objects and relationships for reasoning \cite{teney2017Graph, yi2018neural}.  Yi \etal \cite{yi2018neural}  establish structured representations of the images and questions and perform reasoning as symbolic program execution. It's interpretable in the reasoning process, but still ignoring the relational visual clues.  \cite{teney2017Graph} builds scene graphs over the objects and encodes relative spatial relationships, which is limited by the expressive ability of the simple spatial relationships. Our work goes one step further by modeling the visual content by relation-aware scene graph, language-guided visual relationships, and integrating them with the explicitly-interpretable graph convolutional networks for visual reasoning. 

\subsection{Detailed Model Architecture}

\subsection{Experimental Details}

\subsection{Additional Qualitative Results}

Shown in Fig.\ref{fig:vis_2}. For each question, column \textit{a} shows the original image; column \textit{b} depicts the distribution of the question-relation guided self-attention with respect to the object attended by the question guided object attention (the relation label is predicted by the visual relationship encoder); column \textit{c} shows the distribution of the question guided object attention.

\begin{figure}
\centering
\includegraphics[width=\textwidth]{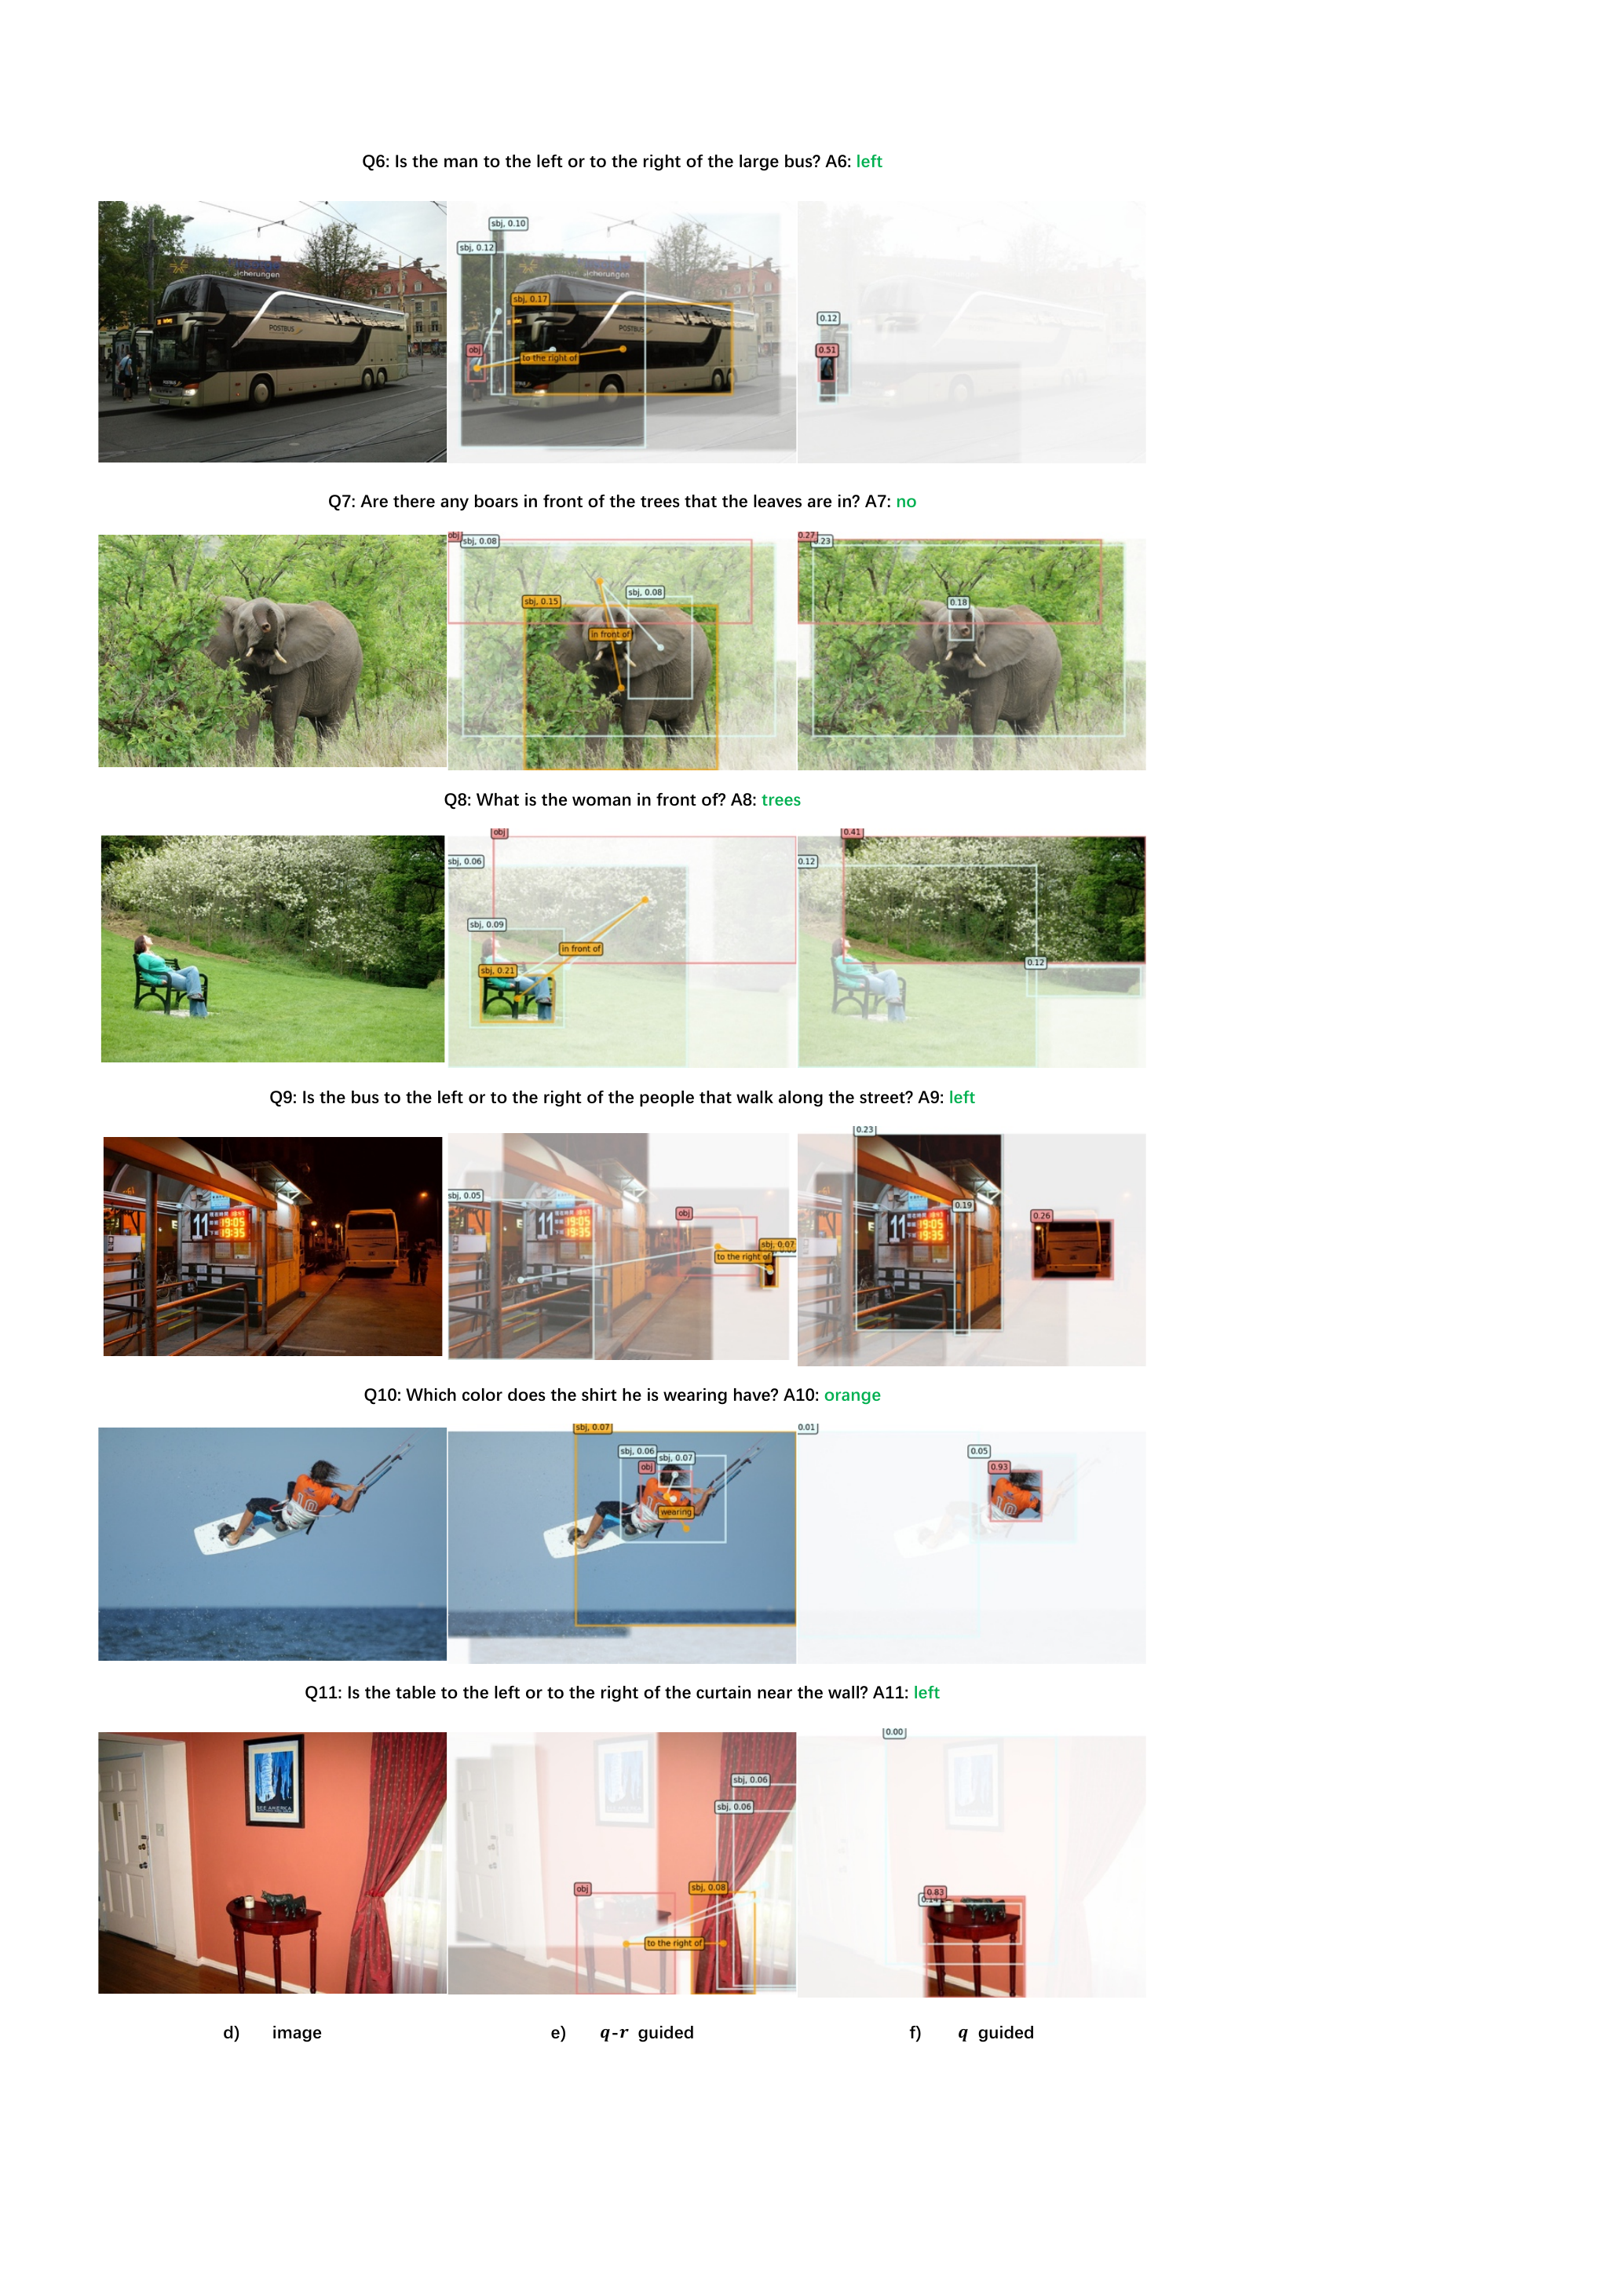} 
\caption{Additional visualization results. Please enlarge to see details.}
\label{fig:vis_2}

\end{figure}
